# Supplementary material for: From Literature to Hypotheses: An AI Co-Scientist System for Biomarker-Guided Drug Combination Hypothesis Generation
Source: arXiv:2603.00612 source file (2026-10-01)
Supplement: Supplementary file 1 [file Appendix.tex]

\appendix
\section{Databases}\label{sec:datasets}
The list of Bioinformatics and Pharmacology-
ical Databases used to construct the Knowledge Graph is in Table \ref{tab1:bio_databases}.
\input{images/dataset}

\section{Example Task-Specific Knowledge Graph}
\label{sec:appendix_kg}

Figure~\ref{fig:kg_example} shows an example task-specific knowledge graph constructed by CoDHy for a single scenario. Node colors indicate entity types, and edges represent typed relations integrated from curated databases and PubMed-derived evidence. This graph is used for embedding generation and evidence-grounded hypothesis construction.

\begin{figure}[t]
\centering
\includegraphics[width=\columnwidth, trim=3cm 1.5cm 4cm 1cm]{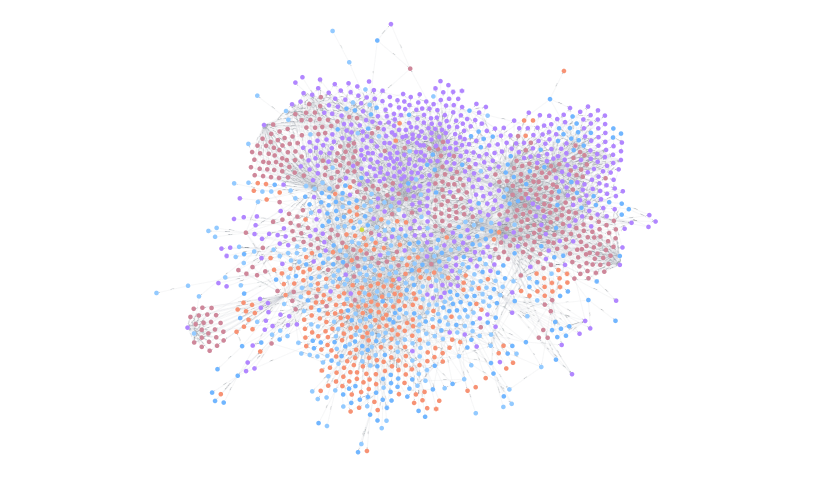}
\caption{\textbf{Example task-specific knowledge graph.} Node colors denote entity types (e.g., gene, drug, disease, variant etc.), and edges correspond to integrated biomedical relations used by CoDHy.}
\label{fig:kg_example}
\end{figure}

\section{Evaluation Scenarios} \label{sec:appendix-scenarios}
Table~\ref{tab2:eval_scenario} lists the fixed set of evaluation scenarios used in all experiments. Each scenario is defined by a cancer type and a focus biomarker and is held constant across all compared methods to ensure fair and consistent evaluation.
\input{images/senarios}

\section{Evaluation Metric Definitions}
\label{sec:metric-definitions}

\paragraph{Novelty.}
\emph{Novel-exact}: no PubMed hits for ``DrugA AND DrugB''.  
\emph{Novel-in-context}: no hits for ``DrugA AND DrugB AND CancerType''.  
Reported as proportions averaged across scenarios.

\paragraph{Evidence Coverage.}
Proportion of hypotheses with $\ge 1$ supporting PubMed reference.

\paragraph{Proceed@\textit{k}.}
Proportion of scenarios where at least one \emph{Proceed} hypothesis appears in the top-\textit{k} (k=1,3).

\paragraph{Diversity.}
Average number of unique drug pairs generated per scenario.

\paragraph{MRR.}
Mean reciprocal rank of the highest-ranked non-zero relevance hypothesis.

\paragraph{nDCG@3.}
Normalized DCG over the top 3 hypotheses using relevance labels
(\emph{Literature Supported} = 1, \emph{Novel/Unsupported} = 0).


\section{Full Demo Outputs}
\label{sec:appendix_outputs}

This appendix provides full structured outputs for two representative use cases generated by the Full CoDHy system. Each scenario includes the four ranked hypotheses as returned by the demo interface, including mechanism description, rationale type, validation verdict, and supporting evidence links. 
In addition to the representative use cases presented here, all experimental logs, extended scenario outputs, and additional reports are provided in structured JSON format in our public GitHub repository.

\subsection{Use Case A: (Breast Invasive Carcinoma, EGFR)}
\label{sec:appendix_egfr}

\paragraph{H1 — Afatinib + Palbociclib}
\textbf{Score:} 9.0 \quad
\textbf{Verdict:} Proceed  
\textbf{Rationale Type:} Direct Graph Evidence  
\textbf{Mechanism:} Resistance reversal via EGFR inhibition and CDK4/6 blockade.  
\textbf{Supporting Evidence:} PMIDs 41723568, 41723552, 41723543, 41723513, 41723496
\textbf{Evidence Status:} Validated (Literature Exists)  
\textbf{Safety Score:} 8  
\textbf{Toxicity Risk:} Moderate (overlapping dermatologic and gastrointestinal toxicities).

\medskip

\paragraph{H2 — Lapatinib + AZD9291}
\textbf{Score:} 9.0 \quad
\textbf{Verdict:} Caution  
\textbf{Rationale Type:} Inferred Similarity  
\textbf{Mechanism:} Synthetic lethality through EGFR amplification and dual pathway inhibition.  
\textbf{Supporting Evidence:} PMIDs 32547705, 29103264  
\textbf{Evidence Status:} Validated (Literature Exists)  
\textbf{Safety Score:} 8  
\textbf{Toxicity Risk:} Moderate (predicted overlapping toxicities).

\medskip

\paragraph{H3 — Osimertinib + Fulvestrant}
\textbf{Score:} 9.0 \quad
\textbf{Verdict:} Proceed  
\textbf{Rationale Type:} Inferred Similarity  
\textbf{Mechanism:} Estrogen-dependent synthetic lethality combined with EGFR inhibition.  
\textbf{Supporting Evidence:} PMIDs 41723568, 41723543  
\textbf{Evidence Status:} Validated (Literature Exists)  
\textbf{Safety Score:} 8  
\textbf{Toxicity Risk:} Moderate.

\medskip

\paragraph{H4 — Ceritinib + Everolimus}
\textbf{Score:} 9.0 \quad
\textbf{Verdict:} Proceed  
\textbf{Rationale Type:} Direct Graph Evidence  
\textbf{Mechanism:} Resistance reversal via mTOR pathway inhibition.  
\textbf{Supporting Evidence:} PMIDs 41706704, 41622283  
\textbf{Evidence Status:} Validated (Literature Exists)  
\textbf{Safety Score:} 8  
\textbf{Toxicity Risk:} Moderate.

\subsection{Use Case B: (Breast Invasive Carcinoma, PIK3CA)}
\label{sec:appendix_pik3ca}

\paragraph{H1 — Palbociclib + Everolimus}
\textbf{Score:} 5.0 \quad
\textbf{Verdict:} Reject  
\textbf{Rationale Type:} Direct Graph Evidence  
\textbf{Mechanism:} Synthetic lethality via CDK4/6–PIK3CA interaction and mTOR inhibition.  
\textbf{Supporting Evidence:} PMIDs 41647714, 41617434, 41594421  
\textbf{Evidence Status:} Validated (Literature Exists)  
\textbf{Safety Score:} 8  
\textbf{Toxicity Risk:} Moderate (hepatotoxicity and gastrointestinal effects).

\medskip

\paragraph{H2 — Alpelisib + Temozolomide}
\textbf{Score:} 4.91 \quad
\textbf{Verdict:} Proceed (with Caution)  
\textbf{Rationale Type:} Inferred Similarity  
\textbf{Mechanism:} Synthetic lethality via PI3K inhibition and DNA damage induction.  
\textbf{Supporting Evidence:} PMIDs 41518601, 41372143, 35324454  
\textbf{Evidence Status:} Validated (Literature Exists)  
\textbf{Safety Score:} 8  
\textbf{Toxicity Risk:} Moderate (combined metabolic and neurological risks).

\medskip

\paragraph{H3 — AZD8186 + Everolimus}
\textbf{Score:} 4.8 \quad
\textbf{Verdict:} Proceed (with Caution)  
\textbf{Rationale Type:} Direct Graph Evidence  
\textbf{Mechanism:} Resistance reversal via PI3K–mTOR axis inhibition.  
\textbf{Supporting Evidence:} No direct clinical study found (novel combination)  
\textbf{Evidence Status:} Inferred (Novel Combination)  
\textbf{Safety Score:} 8  
\textbf{Toxicity Risk:} Predicted moderate.

\medskip

\paragraph{H4 — BKM120 + Trametinib}
\textbf{Score:} 4.8 \quad
\textbf{Verdict:} Reject  
\textbf{Rationale Type:} Inferred Similarity  
\textbf{Mechanism:} Synthetic lethality via PI3K and MEK inhibition.  
\textbf{Supporting Evidence:} Preclinical literature references  
\textbf{Evidence Status:} Partially supported  
\textbf{Safety Score:} 8  
\textbf{Toxicity Risk:} Moderate.
